# Supplementary material for: Dirty higher-order Dirac semimetal: Quantum criticality and bulk-boundary correspondence
Source: arXiv:2002.09475 ancillary file (2020-11-09)
Supplement: Supplementary file 1 [file Supplementary.pdf]

# Supplemental Materials: Dirty higher-order Dirac semimetal: Quantum criticality and bulk-boundary correspondence

András L. Szabó[1] and Bitan Roy[2]

[1] *Max-Planck-Institut für Physik komplexer Systeme, Nöthnitzer Str. 38, 01187 Dresden, Germany*
[2] *Department of Physics, Lehigh University, Bethlehem, Pennsylvania, 18015, USA*

The Supplemental Materials contain additional numerical results for disordered HOTDSM, discussed in details in Sec. III and Appendix B of the main text.

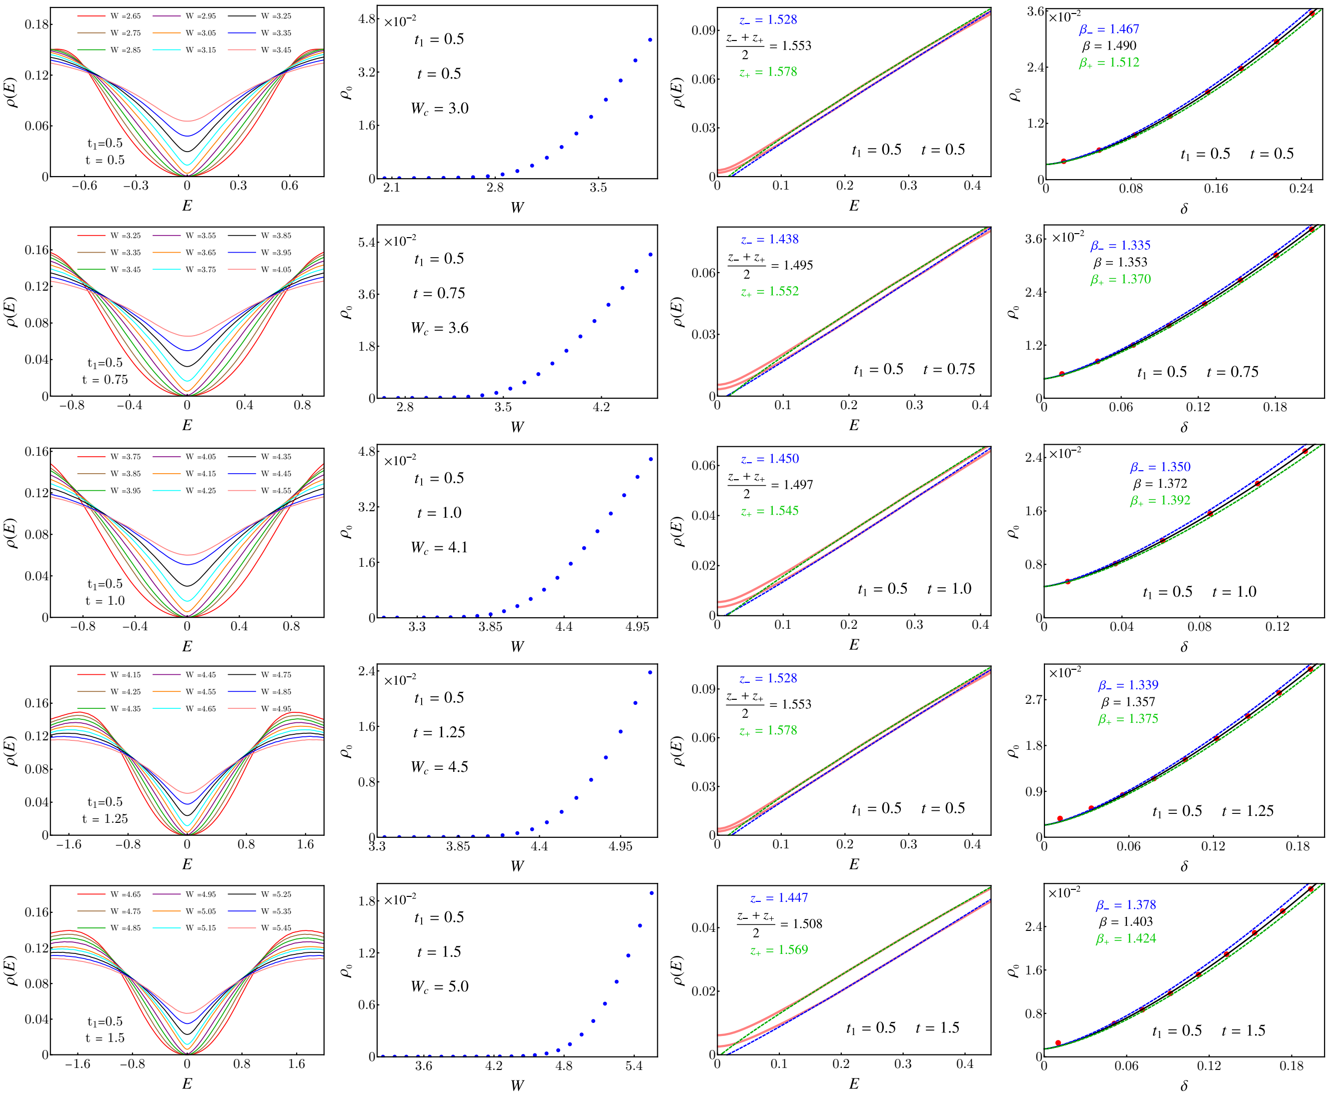


FIG. S1: Scaling analysis of DOS in a HOTDSM (for fixed $t_1 = 0.5$), see Appendix B of the main text for details. For fixed $t_1$, as $t$ (or Fermi velocity) increases, $W_c$ increases. Comparing Fig. 5 of the main text and Figs. S1-S4, we note that for any fixed $t$ (or Fermi velocity) as $t_1$ (determining the strength of the $C_4$ symmetry breaking Wilson mass, yielding the HOTDSM) increases, the DOS decreases at low energies, without altering $\rho(E) \sim |E|^2$. Concomitantly, for fixed $t$ the critical disorder $W_c$ for metallicity increases with increasing $t_1$.

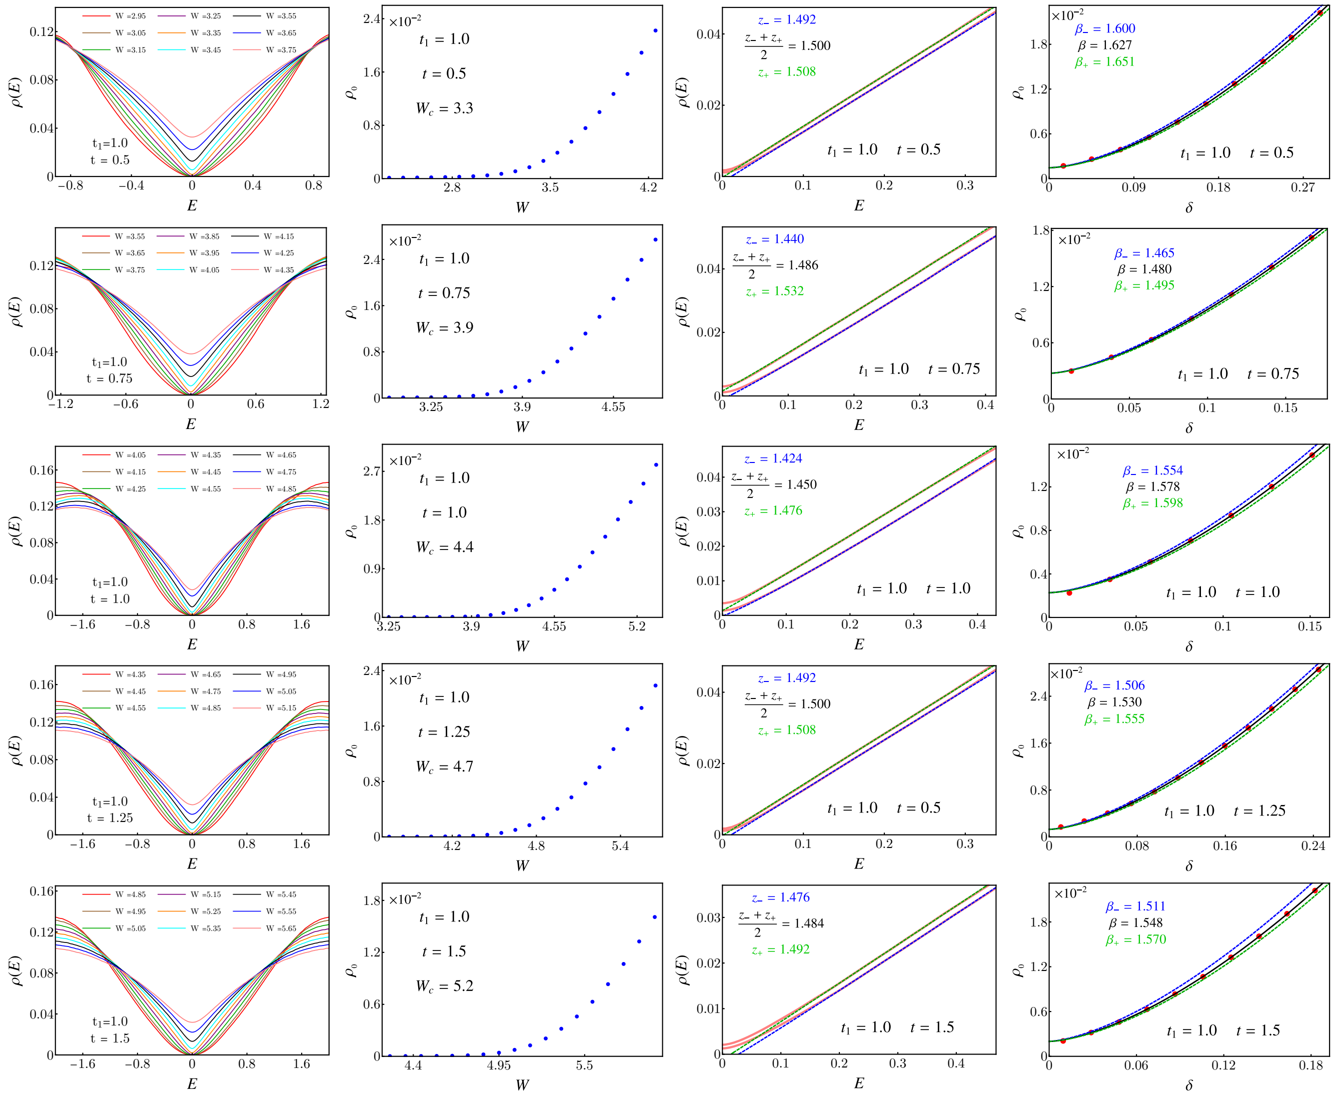

FIG. S2: Scaling analysis of DOS in a HOTDSM (for fixed $t_1 = 1.0$), see Appendix B of the main text for details. Once again for fixed $t_1$, as $t$ (or Fermi velocity) increases, $W_c$ increases.

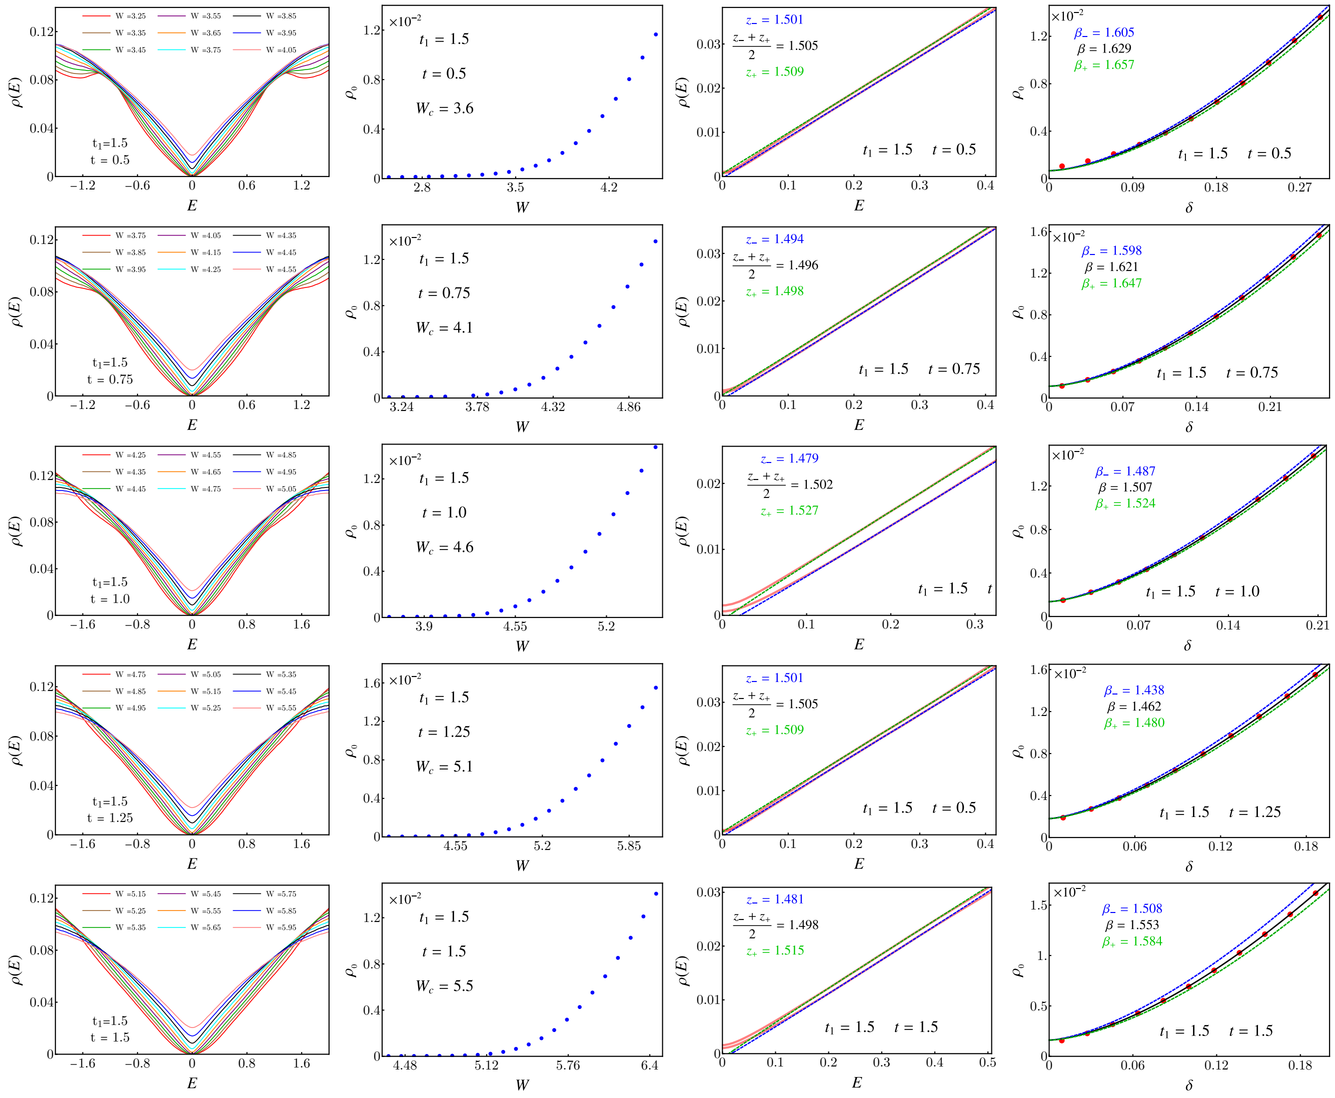

FIG. S3: Scaling analysis of DOS in a HOTDSM (for fixed $t_1 = 1.5$), see Appendix B of the main text for details. Once again for fixed $t_1$, as $t$ (or Fermi velocity) increases, $W_c$ increases.

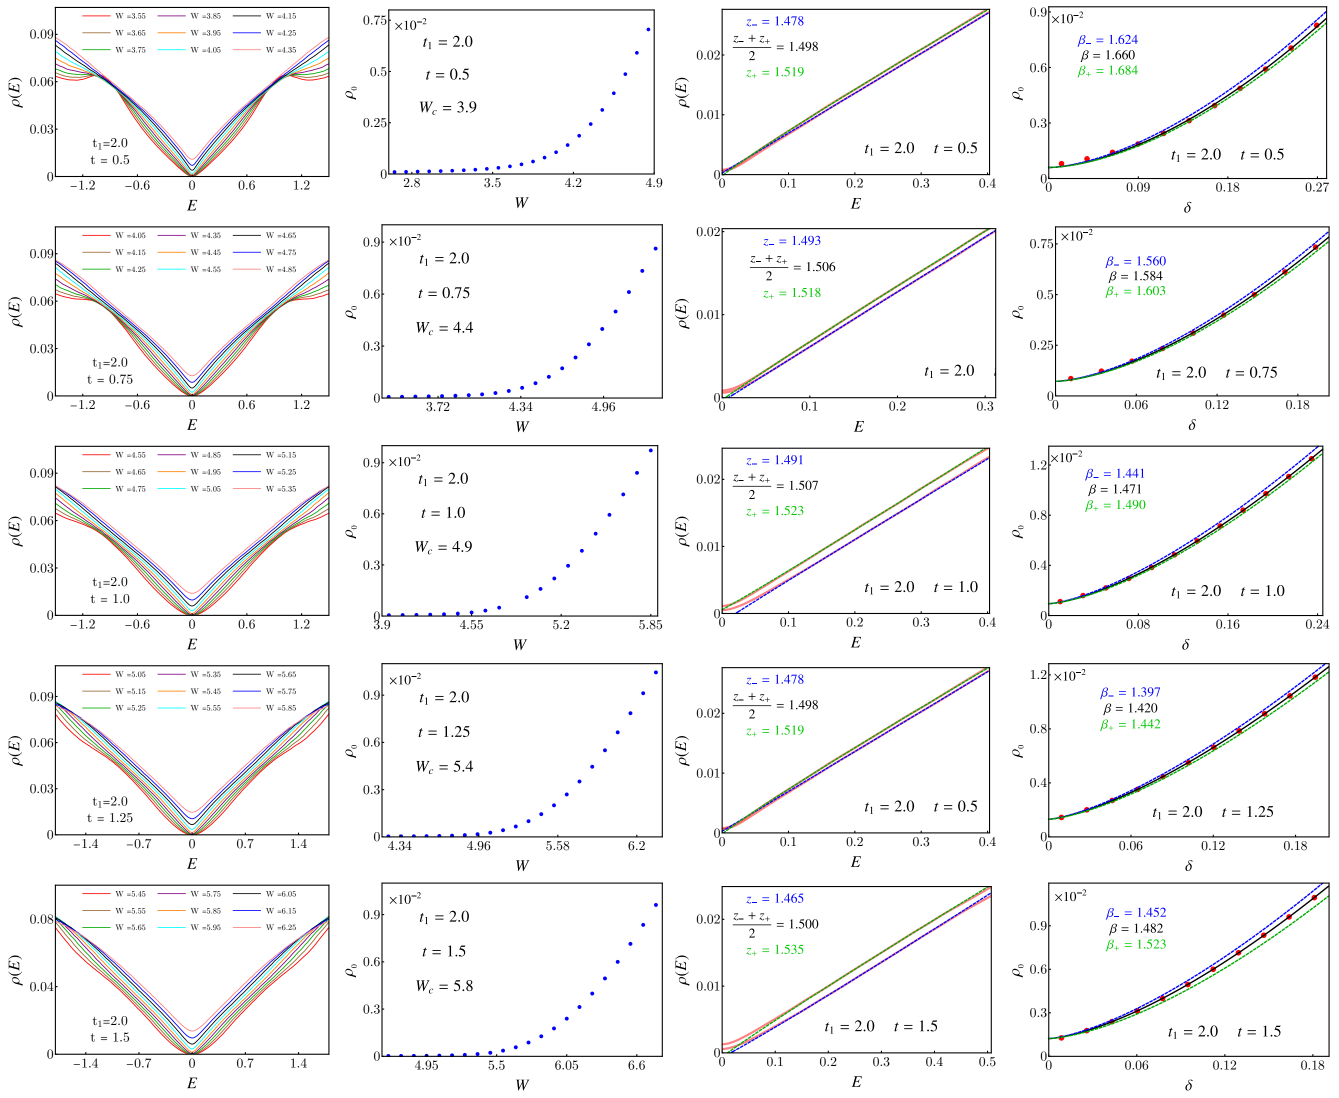

FIG. S4: Scaling analysis of DOS in a HOTDSM (for fixed $t_1 = 2.0$), see Appendix B of the main text for details. Once again for fixed $t_1$, as $t$ (or Fermi velocity) increases, $W_c$ increases.
